# Supplementary material for: Demonstration of microwave single-shot quantum key distribution
Source: arXiv:2311.11069 ancillary file (2023-11-18)
Supplement: Supplementary file 1 [file FF_CVQKD_SuppInfo.pdf]

# Supplementary Information for "Demonstration of microwave single-shot quantum key distribution"

F. Fesquet,[1,2,*] F. Kronowetter,[1,2,3] M. Renger,[1,2] W. K. Yam,[1,2] S. Gandorfer,[1,2]
K. Inomata,[4,5] Y. Nakamura,[4,6] A. Marx,[1] R. Gross,[1,2,7] and K. G. Fedorov[1,2,7,†]

[1]*Walther-Meißner-Institut, Bayerische Akademie der Wissenschaften, 85748 Garching, Germany*
[2]*School of Natural Sciences, Technische Universität München, 85748 Garching, Germany*
[3]*Rohde & Schwarz GmbH & Co. KG, 81671 Munich, Germany*
[4]*RIKEN Center for Quantum Computing (RQC), Wako, Saitama 351-0198, Japan*
[5]*National Institute of Advanced Industrial Science and Technology, 1-1-1 Umezono, Tsukuba, Ibaraki, 305-8563, Japan*
[6]*Department of Applied Physics, Graduate School of Engineering, The University of Tokyo, Bunkyo-ku, Tokyo 113-8656, Japan*
[7]*Munich Center for Quantum Science and Technology (MCQST), 80799 Munich, Germany*

## I. EXPERIMENTAL SETUP

The cryogenic and the room-temperature setups are shown in Fig. S1. Both Josephson parametric amplifiers (JPAs) are pumped with a microwave signal source (SGS 100A from Rohde & Schwarz). During measurements with only a single JPA, the other JPA is detuned far from resonance (typically by several dozens of megahertz) using a dc magnetic flux bias provided by a superconducting solenoid installed on top of each JPA sample box. This frequency detuning prevents the JPAs from interfering with each other during individual measurements. Additionally, each JPA is encapsulated by an aluminum box to prevent magnetic flux crosstalk between the JPAs at cryogenic temperatures. The noise coupled to the second directional coupler is generated by an arbitrary waveform generator (AWG) acting as a Gaussian noise source (AWG 81160A from Keysight). This Gaussian noise has a bandwidth of $200\,\mathrm{MHz}$ and is up-converted to signal frequencies (around $5\,\mathrm{GHz}$) using an radio frequency (RF) source. The output signal after the high-electron-mobility transistor (HEMT, LNF-LNC4_8F from Low Noise Factory) is amplified by a room-temperature RF amplifier (AMT-A0033 from Agile MwT). We use a vector network analyzer (VNA) for spectroscopic measurements of both JPAs and to characterise their magnetic flux-dependent frequency. State tomography is performed with a room-temperature heterodyne detection setup, as presented in ref. S1, S2. Amplified signals are filtered around the center frequency using a bandpass filter before being down-converted to an intermediate frequency (IF) signal of $12.5\,\mathrm{MHz}$ with a local oscillator. The resulting IF signals are filtered before being amplified by a room-temperature IF amplifier (AU-1447 from Miteq). The subsequent signals are digitized using an analog-to-digital converter (ADC) integrated in a National Instruments NI-5782 transceiver module and processed with a National Instruments PXIe-7972 field-programmable gate array (FPGA) module. The data processing, resulting in *I/Q* sampled data points, consists of a digital downconversion (DDC) and a filtering using a digital finite-impulse response (FIR) filter with a full measurement bandwidth of $400\,\mathrm{kHz}$. For state tomography, we compute the quadrature moments $\langle I^n Q^m \rangle$ for $n+m \leq 4$ $[(n,m) \in \mathbb{N}^2]$ from $2.475\times10^8$ filtered *I/Q* points. The quadrature

* florian.fesquet@wmi.badw.de
† kirill.fedorov@wmi.badw.de

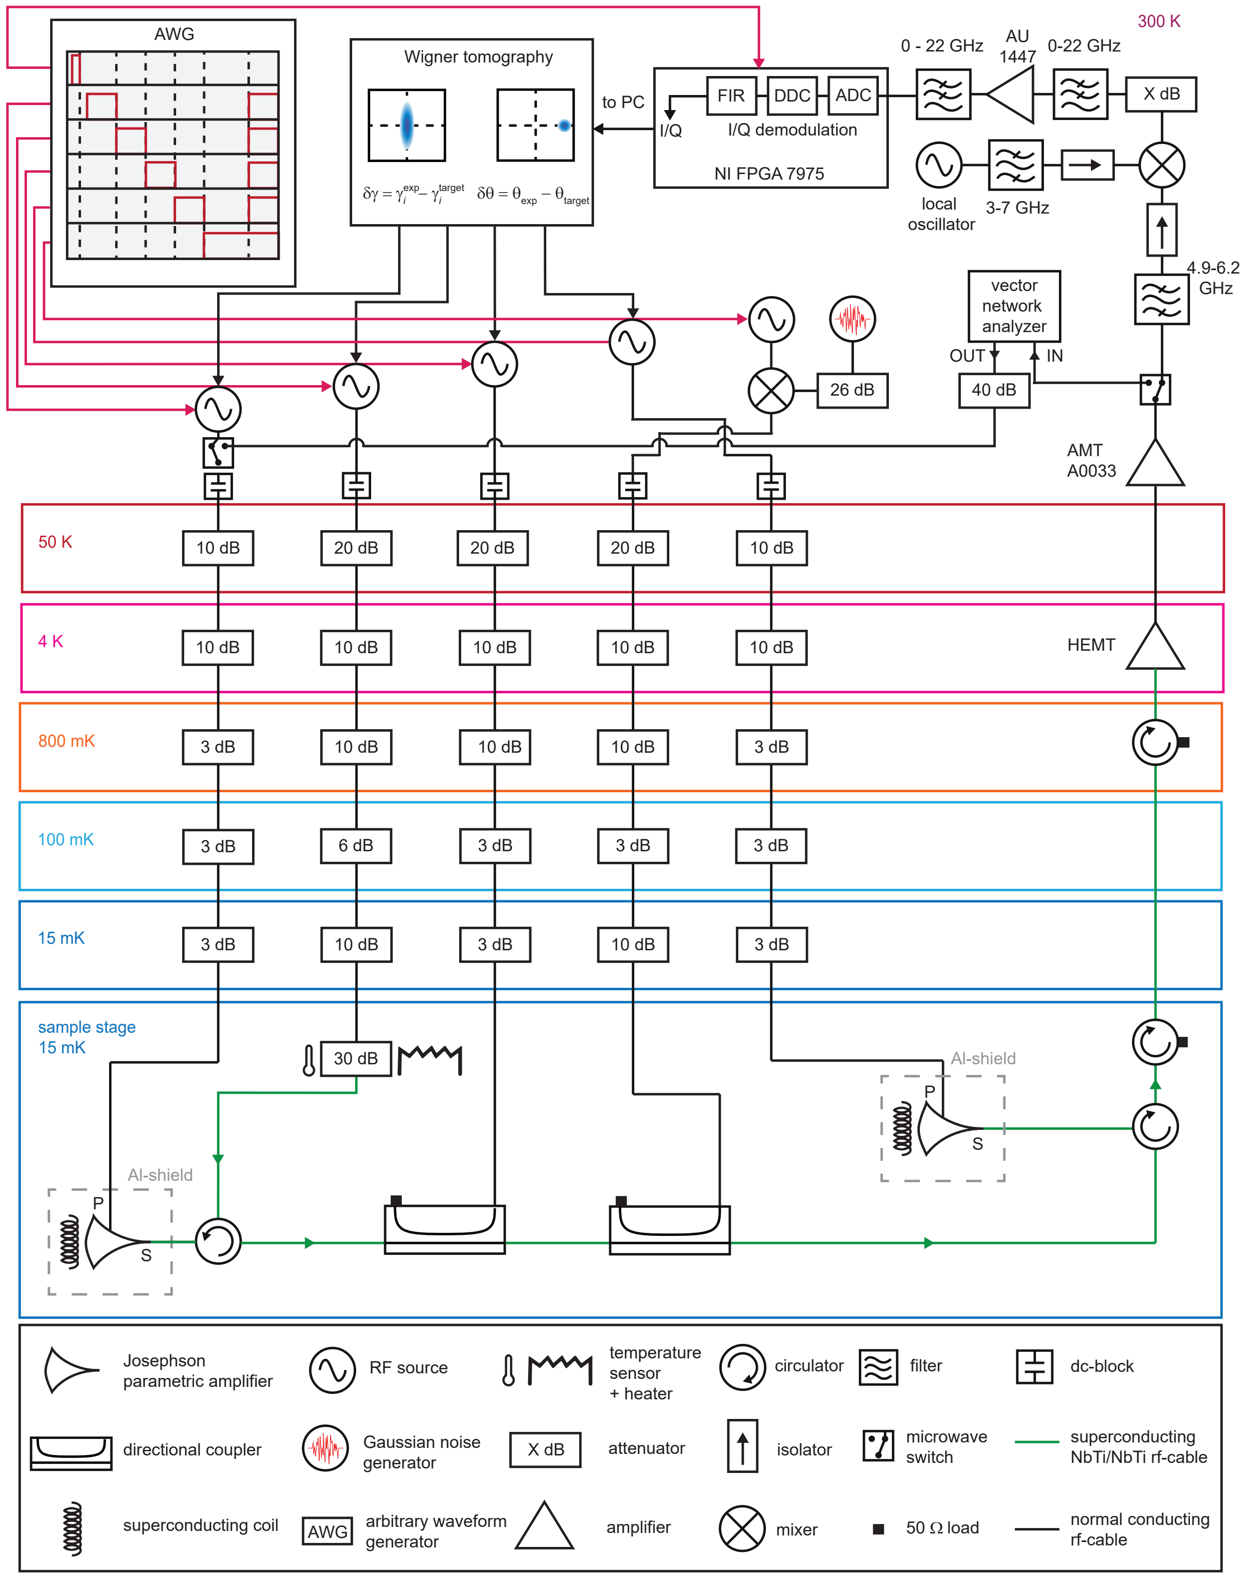


Figure S1. Experimental scheme of our CV-QKD implementation with propagating microwave states. The superconducting magnetic coils are located on top of the JPAs. All microwave signal sources are pulsed using an AWG.

moments of the JPAs are used to compute the signal moments $\langle(\hat{a}^\dagger)^n\hat{a}^m\rangle$ with the reference-state reconstruction method [S1, S3]. The moments are reconstructed with respect to a specific reconstruction point in our setup, which can be freely moved. Using this method, we reconstruct experimental squeezing angles $\gamma_i^{\exp}$ ($i \in \{1,2\}$) for each JPA and compute angle corrections, which are used to adjust the phase of the pump tones of the JPAs by $2\delta\gamma = 2(\gamma_i^{\exp} - \gamma_i^{\text{target}})$. A similar procedure is followed to reconstruct a displacement angle and adjust the phase of the coherent tone sent to the first directional coupler by $\delta\theta = \theta_{\exp} - \theta_{\text{target}}$. This procedure ensures a stable phase of all signals during our measurements. For state tomography, the angles are continuously adjusted. For single-shot measurements, we restrict our data analysis to single *I/Q* points and do not continuously adjust the phase of the signal sources. Instead, we measure the phase drift of our signal sources and adjust the phases only when the symbol chosen by Alice is changed. Knowing the signal phase drift, we ensure that the phase remains stable within less than 1 degree during the single-shot measurements. For our reference-state reconstruction method, we switch on our devices during precise time windows of our data acquisition measurement window. This is achieved using another AWG (HDAWG from Zurich Instruments), which generates square pulses to periodically trigger our devices for a given time window. This HDAWG additionally provides a trigger signal for the FPGA card for a proper synchronization of the data acquisition and the devices. The VNA, HDAWG, FPGA, and local oscillator are synchronized by a $10\,\text{MHz}$ reference signal from a rubidium frequency standard. The microwave signal sources are daisy chained to the local oscillator with a $1\,\text{GHz}$ reference signal. During state tomography measurements, we compute cumulants up to the forth order to verify the Gaussianity of our quantum states [S2].

## II. QUADRATURE DISTRIBUTION MODEL

The scheme of our CV-QKD implementation setup is shown in Fig. S2. It consists of one main signal path and two additional paths to account for the signals sent to the directional couplers. We divide our setup into multiple segments. For each segment, we introduce an operator acting on the signal modes, denoted $\hat{a}_1$. The modes for the two other paths are denoted as $\hat{a}_2$ and $\hat{a}_3$, respectively. The weak thermal environment in each segment is modelled as a bosonic mode with an average noise photon number

$$\bar{n}_{\text{th}} = \frac{1}{\exp\left(\frac{\hbar\omega}{k_{\text{B}}T}\right) - 1}. \tag{S1}$$

The squeezing operation implemented by the first JPA, corresponding to Alice, is described by a squeeze operator $\hat{S}_{\text{A}} = \exp[(\xi^*\hat{a}_1^2 - \xi(\hat{a}_1^\dagger)^2)/2]$. This operator is parametrized by a squeeze factor $r_{\text{A}} = |\xi|$ and a squeezing angle $\varphi_{\text{A}} = \arg(\xi)$, which determines the amplitude and the direction of the squeezing operation. The action of the squeeze operator on a signal mode results in the transformation

$$\hat{S}_{\text{A}}^\dagger\hat{a}_1\hat{S}_{\text{A}} = \hat{a}_1\cosh(r_{\text{A}}) - \hat{a}_1^\dagger\sinh(r_{\text{A}})e^{-2i\varphi_{\text{A}}}. \tag{S2}$$

Alice performs this squeezing operation along the $q$ quadrature (for $\varphi_{\text{A}} = 0$) or the $p$ quadrature (for $\varphi_{\text{A}} = \pi$). For a given symbol $\alpha_i$, each squeezed state is displaced in quadrature phase space by applying the displacement operator $\hat{D}(\alpha_i) = \exp\left(\alpha_i\hat{a}_1^\dagger - \alpha_i^*\hat{a}_1\right)$ resulting in the transformation of an input signal mode $\hat{a}_1$ as

$$\hat{a}_1^{'} = \hat{D}^\dagger(\alpha_i)\,\hat{a}_1\hat{D}(\alpha_i) = \hat{a}_1 + \alpha_i. \tag{S3}$$

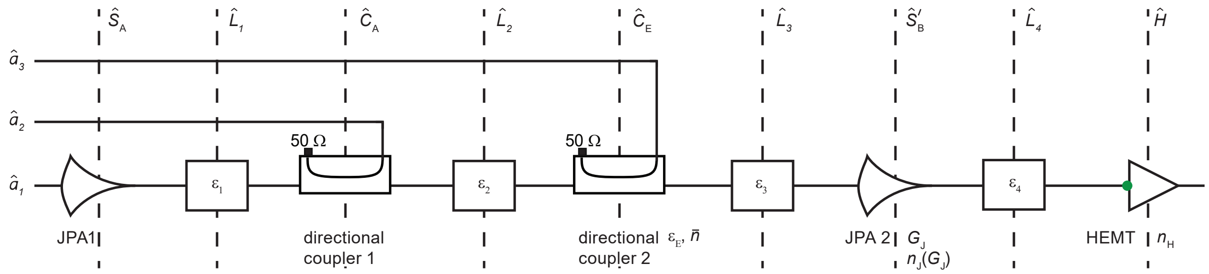


Figure S2. Scheme for the theoretical modelling of the CV-QKD protocol implementation. The setup is split into several segments and consists of three paths. Each segment has either an operation on path signal ($\hat{S}_\mathrm{A}$, $\hat{S}'_\mathrm{B}$) or between path signals ($\hat{C}_\mathrm{A}$, $\hat{C}_\mathrm{E}$), or path losses ($\hat{L}_1$,$\hat{L}_1$, $\hat{L}_2$, $\hat{L}_3$, $\hat{L}_4$) and added noise ($\hat{H}$). The second directional coupler is characterized by the losses $\varepsilon_\mathrm{E}$ and coupled noise photon number $\bar{n}$. For our model, the output state is effectively reconstructed at the input of the HEMT (while accounting for the HEMT noise), indicated by a green dot. Here, we do not show the modes corresponding to the path losses and HEMT noise.

This displacement operation is realized by the first directional coupler, acting as a highly asymmetric beamsplitter with a power transmissivity $\tau_\mathrm{A}$, described as

$$\hat{C}^\dagger_\mathrm{A}\left(\tau_\mathrm{A}\right)\begin{pmatrix}\hat{a}_1\\ \hat{a}_2\end{pmatrix}\hat{C}_\mathrm{A}\left(\tau_\mathrm{A}\right)=\begin{pmatrix}\sqrt{\tau_\mathrm{A}}\,\hat{a}_1+\sqrt{1-\tau_\mathrm{A}}\,\hat{a}_2\\ -\sqrt{1-\tau_\mathrm{A}}\,\hat{a}_1+\sqrt{\tau_\mathrm{A}}\,\hat{a}_2\end{pmatrix}. \tag{S4}$$

The coupling of $\bar{n}$ noise photons to Alice's signals is performed using the second directional coupler which we model with a beamsplitter of transmissivity $\tau_\mathrm{E}=1-\varepsilon_\mathrm{E}$, resulting in

$$\hat{C}^\dagger_\mathrm{E}\left(\varepsilon_\mathrm{E}\right)\begin{pmatrix}\hat{a}_1\\ \hat{a}_2\end{pmatrix}\hat{C}_\mathrm{E}\left(\varepsilon_\mathrm{E}\right)=\begin{pmatrix}\sqrt{1-\varepsilon_\mathrm{E}}\,\hat{a}_1+\sqrt{\varepsilon_\mathrm{E}}\,\hat{a}_2\\ -\sqrt{\varepsilon_\mathrm{E}}\,\hat{a}_1+\sqrt{1-\varepsilon_\mathrm{E}}\,\hat{a}_2\end{pmatrix}. \tag{S5}$$

The path losses in the different sections of the setup are modelled using a beamsplitter model

$$\hat{L}^\dagger_j\hat{a}_1\hat{L}_j=\sqrt{1-\varepsilon_j}\,\hat{a}_1+\sqrt{\varepsilon_j}\,\hat{h}_j, \tag{S6}$$

with $j\in\{1,2,3,4\}$. The bosonic modes $\hat{h}_j$ model the thermal environment with a mean thermal photon number $\bar{n}_\mathrm{th}$. Lastly, we describe the phase-sensitive amplification of the measurement JPA (second JPA) using a noisy squeeze operator to account for the amplification noise added by the JPA itself. We introduce a classical complex random variable $\zeta$ to model the added noise such that

$$(\hat{S}'_\mathrm{B})^\dagger\hat{a}_1\hat{S}'_\mathrm{B}=(\hat{a}_1+\zeta)\cosh(r_\mathrm{B})-(\hat{a}^\dagger_1+\zeta^*)\sinh(r_\mathrm{B})e^{-2i\varphi_\mathrm{B}}, \tag{S7}$$

where $\zeta$ satisfies $\langle|\zeta|^2\rangle=\bar{n}_\mathrm{J}$. We assume an even splitting of the noise between the $q$ and $p$ quadrature, $\langle\mathrm{Re}\,(\zeta)^2\rangle=\langle\mathrm{Im}\,(\zeta)^2\rangle=\bar{n}_\mathrm{J}/2$, and that $\zeta$ has a zero-mean Gaussian distribution [S2]. The noise of the JPA depends on the JPA gain $G_\mathrm{J}$ as

$$\bar{n}_\mathrm{J}\left(G_\mathrm{J}\right)=\Xi_1\left(G_\mathrm{J}-1\right)^{\Xi_2}, \tag{S8}$$

where $\Xi_1$ and $\Xi_2$ are phenomenological constants characterizing the noise properties of the JPA. Since we are considering single-shot measurements, we account for the phase-insensitive amplifi-

cation performed by the HEMT, which we describe as

$$\hat{H}^\dagger \hat{a}_1 \hat{H} = \sqrt{G_\mathrm{H}}\,\hat{a}_1 + \sqrt{G_\mathrm{H}-1}\,\hat{h}_\mathrm{H}^\dagger. \tag{S9}$$

Here, $\hat{h}_\mathrm{H}$ is a thermal mode with a mean photon number $\bar{n}_\mathrm{H}$ describing the added HEMT noise and $G_\mathrm{H}$ is the HEMT amplification gain. We note that this would imply that signal moments are reconstructed at the output of the HEMT. In the measurements, we ultimately shift this reconstruction point to the input of the HEMT by rescaling the measured data by the HEMT gain. The full protocol implementation is expressed by the operator $\hat{T}$ as

$$\hat{T} = \hat{H}\hat{L}_4\hat{S}'_\mathrm{B}\hat{L}_3\hat{C}_\mathrm{E}\hat{L}_2\hat{C}_A\hat{L}_1\hat{S}_\mathrm{A}. \tag{S10}$$

We write the overall input state of our experimental setup as

$$\hat{\rho}_\mathrm{in} = \hat{\rho}_1 \otimes \hat{\rho}_2 \otimes \hat{\rho}_3, \tag{S11}$$

where the states $\hat{\rho}_i$ describe the signal in path $i$ with $i \in \{1,2,3\}$. The input signal in path $1$ is modelled as a weak thermal state with a thermal population $\bar{n}_\mathrm{th}$. The input signal in the path $2$ is described as a strongly displaced thermal state, to account for the thermal background noise photons $\bar{n}_\mathrm{th}$. Lastly, the input signal in path $3$ corresponds to a strong Gaussian noise with an averaged photon number $\bar{n}_\mathrm{E}$, which couples to the second directional coupler. We note that a more complete description of our system would lead to

$$\hat{\rho}_\mathrm{in} = \hat{\rho}_1 \otimes \hat{\rho}_2 \otimes \hat{\rho}_3 \otimes \hat{\rho}_\mathrm{th}^{\otimes 4} \otimes \hat{\rho}_\mathrm{H}, \tag{S12}$$

where $\hat{\rho}_\mathrm{th}$ is a thermal state with an average thermal population $\bar{n}_\mathrm{th}$ associated with the path loss operators $\hat{L}_j$ with $j \in \{1,2,3,4\}$. Additionally, $\hat{\rho}_\mathrm{H}$ is a thermal state associated with the HEMT operator $\hat{H}$. In the following expressions for displacement vectors and covariance matrices, we implicitly do not consider these additional modes in our quantum model in order to keep the dimension of the system small. We emphasize that the results of our model remain entirely unchanged by this truncation. Therefore, we use Eq. S11, to describe our system. The final output state after the HEMT can be expressed as

$$\hat{\rho}_\mathrm{out} = \hat{T}\hat{\rho}_\mathrm{in}\hat{T}^\dagger. \tag{S13}$$

The moments of the output signals $\hat{b}_i$ (signals at the output of the end of our device chain) can be calculated as

$$\begin{pmatrix} \langle (\hat{b}_1^\dagger)^n \hat{b}_1^m \rangle \\ \langle (\hat{b}_2^\dagger)^n \hat{b}_2^m \rangle \\ \langle (\hat{b}_3^\dagger)^n \hat{b}_3^m \rangle \end{pmatrix} = \begin{pmatrix} \mathrm{Tr}((\hat{a}_1^\dagger)^n \hat{a}_1^m \hat{\rho}_\mathrm{out}) \\ \mathrm{Tr}((\hat{a}_2^\dagger)^n \hat{a}_2^m \hat{\rho}_\mathrm{out}) \\ \mathrm{Tr}((\hat{a}_3^\dagger)^n \hat{a}_3^m \hat{\rho}_\mathrm{out}) \end{pmatrix}. \tag{S14}$$

Experimentally, we restrict our measurements to the fourth order, i.e., $m+n \leq 4$ with $(m,n) \in \mathbb{N}^2$. With the complementary quadrature operators

$$\hat{q}_i = \frac{\hat{b}_i + \hat{b}_i^\dagger}{2}, \quad \hat{p}_i = \frac{\hat{b}_i - \hat{b}_i^\dagger}{2i}, \tag{S15}$$

we define a vector $\hat{x} = (\hat{q}_1, \hat{p}_1, \hat{q}_2, \hat{p}_2, \hat{q}_3, \hat{p}_3)^\mathrm{T}$. Consider that we use Gaussian states, we fully

describe our Gaussian state using the displacement vector and covariance matrix which read as

$$\begin{gathered} \boldsymbol{d}_{\mathrm{in}} = \langle \hat{x} \rangle \,, \\ \boldsymbol{V}_{\mathrm{in}} = (V_{ij})_{i,j\in D\times D} \,,\; V_{ij} = \langle \hat{x}_i \hat{x}_j + \hat{x}_j \hat{x}_i \rangle /2 - \langle \hat{x}_i \rangle \langle \hat{x}_j \rangle \,, \end{gathered} \tag{S16}$$

where $D = \{1,2,3,4,5,6\}$. According to Eq. S11, for the input state corresponding to $\hat{\rho}_{\mathrm{in}}$ we obtain

$$\begin{gathered} \boldsymbol{d}_{\mathrm{in}} = (0,0,\sqrt{n_{\mathrm{d}}}\cos(\varphi_{\mathrm{d}}),\sqrt{n_{\mathrm{d}}}\sin(\varphi_{\mathrm{d}}),0,0)^{\mathrm{T}} \,, \\ \boldsymbol{V}_{\mathrm{in}} = \frac{1}{4}\begin{pmatrix} (1+2\bar{n}_{\mathrm{th}})\boldsymbol{I}_2 & \boldsymbol{0}_2 & \boldsymbol{0}_2 \\ \boldsymbol{0}_2 & (1+2\bar{n}_{\mathrm{th}})\boldsymbol{I}_2 & \boldsymbol{0}_2 \\ \boldsymbol{0}_2 & \boldsymbol{0}_2 & (1+2\bar{n}_{\mathrm{E}})\boldsymbol{I}_2 \end{pmatrix} . \end{gathered} \tag{S17}$$

Here, $n_{\mathrm{d}}$ is a displacement photon number and $\varphi_{\mathrm{d}}$ a corresponding displacement angle. For a given symbol of Alice, $\alpha_i$, we have $n_{\mathrm{d}} = |\alpha_i|^2/(1-\tau_{\mathrm{A}})$ and $\varphi_{\mathrm{d}} = 0$ ($\varphi_{\mathrm{d}} = \pi/2$) if Alice chooses to encode the displacement along the $q$-quadrature ($p$-quadrature). The squeezing operation for Alice's JPA is modelled by

$$\boldsymbol{J}_{\mathrm{A}} = \boldsymbol{R}_{\mathrm{A}}\boldsymbol{S}_{\mathrm{A}}\boldsymbol{R}_{\mathrm{A}}^{\mathrm{T}},\; \boldsymbol{S}_{\mathrm{A}} = \begin{pmatrix} e^{-r_{\mathrm{A}}} & 0 & 0 & 0 & 0 & 0 \\ 0 & e^{r_{\mathrm{A}}} & 0 & 0 & 0 & 0 \\ 0 & 0 & 1 & 0 & 0 & 0 \\ 0 & 0 & 0 & 1 & 0 & 0 \\ 0 & 0 & 0 & 0 & 1 & 0 \\ 0 & 0 & 0 & 0 & 0 & 1 \end{pmatrix},\; \boldsymbol{R}_{\mathrm{A}} = \begin{pmatrix} \cos(\gamma_{\mathrm{A}}) & \sin(\gamma_{\mathrm{A}}) & 0 & 0 & 0 & 0 \\ -\sin(\gamma_{\mathrm{A}}) & \cos(\gamma_{\mathrm{A}}) & 0 & 0 & 0 & 0 \\ 0 & 0 & 1 & 0 & 0 & 0 \\ 0 & 0 & 0 & 1 & 0 & 0 \\ 0 & 0 & 0 & 0 & 1 & 0 \\ 0 & 0 & 0 & 0 & 0 & 1 \end{pmatrix} . \tag{S18}$$

The beamsplitter operations are expressed as

$$\boldsymbol{C}_{\mathrm{A}} = \begin{pmatrix} \sqrt{\tau_{\mathrm{A}}}\,\boldsymbol{I}_2 & \sqrt{1-\tau_{\mathrm{A}}}\,\boldsymbol{I}_2 & \boldsymbol{0}_2 \\ -\sqrt{1-\tau_{\mathrm{A}}}\,\boldsymbol{I}_2 & \sqrt{\tau_{\mathrm{A}}}\,\boldsymbol{I}_2 & \boldsymbol{0}_2 \\ \boldsymbol{0}_2 & \boldsymbol{0}_2 & \boldsymbol{I}_2 \end{pmatrix},\; \boldsymbol{C}_{\mathrm{E}} = \begin{pmatrix} \sqrt{1-\varepsilon_{\mathrm{E}}}\,\boldsymbol{I}_2 & \boldsymbol{0}_2 & \sqrt{\varepsilon_{\mathrm{E}}}\,\boldsymbol{I}_2 \\ \boldsymbol{0}_2 & \boldsymbol{I}_2 & \boldsymbol{0}_2 \\ -\sqrt{\varepsilon_{\mathrm{E}}}\,\boldsymbol{I}_2 & \boldsymbol{0}_2 & \sqrt{1-\varepsilon_{\mathrm{E}}}\,\boldsymbol{I}_2 \end{pmatrix} . \tag{S19}$$

The losses are described using two matrices

$$\boldsymbol{L}_j = \begin{pmatrix} \sqrt{1-\varepsilon_j}\,\boldsymbol{I}_2 & \boldsymbol{0}_2 & \boldsymbol{0}_2 \\ \boldsymbol{0}_2 & \boldsymbol{I}_2 & \boldsymbol{0}_2 \\ \boldsymbol{0}_2 & \boldsymbol{0}_2 & \boldsymbol{I}_2 \end{pmatrix},\; \boldsymbol{N}_j = \frac{1}{4}(1+2\bar{n}_{\mathrm{th}}) \begin{pmatrix} \varepsilon_j\boldsymbol{I}_2 & \boldsymbol{0}_2 & \boldsymbol{0}_2 \\ \boldsymbol{0}_2 & \boldsymbol{I}_2 & \boldsymbol{0}_2 \\ \boldsymbol{0}_2 & \boldsymbol{0}_2 & \boldsymbol{I}_2 \end{pmatrix} . \tag{S20}$$

Lastly, the phase-sensitive amplification of the measurement JPA is described using

$$\boldsymbol{J}_{\mathrm{B}} = \boldsymbol{R}_{\mathrm{B}}\boldsymbol{S}_{\mathrm{B}}\boldsymbol{R}_{\mathrm{B}}^{\mathrm{T}},\; \boldsymbol{S}_{\mathrm{B}} = \begin{pmatrix} \frac{1}{\sqrt{G_{\mathrm{J}}}} & 0 & 0 & 0 & 0 & 0 \\ 0 & \sqrt{G_{\mathrm{J}}} & 0 & 0 & 0 & 0 \\ 0 & 0 & 1 & 0 & 0 & 0 \\ 0 & 0 & 0 & 1 & 0 & 0 \\ 0 & 0 & 0 & 0 & 1 & 0 \\ 0 & 0 & 0 & 0 & 0 & 1 \end{pmatrix},\; \boldsymbol{R}_{\mathrm{B}} = \begin{pmatrix} \cos(\gamma_{\mathrm{B}}) & \sin(\gamma_{\mathrm{B}}) & 0 & 0 & 0 & 0 \\ -\sin(\gamma_{\mathrm{B}}) & \cos(\gamma_{\mathrm{B}}) & 0 & 0 & 0 & 0 \\ 0 & 0 & 1 & 0 & 0 & 0 \\ 0 & 0 & 0 & 1 & 0 & 0 \\ 0 & 0 & 0 & 0 & 1 & 0 \\ 0 & 0 & 0 & 0 & 0 & 1 \end{pmatrix} , \tag{S21}$$

with the JPA added noise

$$\boldsymbol{N}_{\mathrm{J}} = \frac{\bar{n}_{\mathrm{J}}}{2}\begin{pmatrix}\boldsymbol{I}_2 & \boldsymbol{0}_2 & \boldsymbol{0}_2\\ \boldsymbol{0}_2 & \boldsymbol{0}_2 & \boldsymbol{0}_2\\ \boldsymbol{0}_2 & \boldsymbol{0}_2 & \boldsymbol{0}_2\end{pmatrix}. \tag{S22}$$

The phase-insensitive amplification performed by the HEMT is modelled as

$$\boldsymbol{H} = \begin{pmatrix}\sqrt{G_{\mathrm{H}}}\boldsymbol{I}_2 & \boldsymbol{0}_2 & \boldsymbol{0}_2\\ \boldsymbol{0}_2 & \boldsymbol{I}_2 & \boldsymbol{0}_2\\ \boldsymbol{0}_2 & \boldsymbol{0}_2 & \boldsymbol{I}_2\end{pmatrix}, \tag{S23}$$

with the HEMT added noise

$$\boldsymbol{N}_{\mathrm{H}} = \frac{\bar{n}_{\mathrm{H}}}{2}\begin{pmatrix}\boldsymbol{I}_2 & \boldsymbol{0}_2 & \boldsymbol{0}_2\\ \boldsymbol{0}_2 & \boldsymbol{0}_2 & \boldsymbol{0}_2\\ \boldsymbol{0}_2 & \boldsymbol{0}_2 & \boldsymbol{0}_2\end{pmatrix}. \tag{S24}$$

We define the sequence

$$\boldsymbol{T} = \boldsymbol{H}\boldsymbol{L}_4\boldsymbol{J}_{\mathrm{B}}\boldsymbol{L}_3\boldsymbol{C}_{\mathrm{E}}\boldsymbol{L}_2\boldsymbol{C}_{\mathrm{A}}\boldsymbol{L}_1\boldsymbol{J}_{\mathrm{A}}. \tag{S25}$$

The displacement vector and covariance matrix of the final state reads

$$\begin{aligned}\boldsymbol{d}_{\mathrm{out}} &= \boldsymbol{T}\boldsymbol{d}_{\mathrm{in}},\\ \boldsymbol{V}_{\mathrm{out}} &= \boldsymbol{T}\boldsymbol{V}_{\mathrm{in}}\boldsymbol{T}^{\mathrm{T}} + \boldsymbol{N}_{\mathrm{out}},\end{aligned} \tag{S26}$$

where the matrix $\boldsymbol{N}_{\mathrm{out}}$ represents the total noise of the protocol implementation and can be calculated by chaining the different losses and amplification noise contributions. We find the expression

$$\begin{aligned}\boldsymbol{N}_{\mathrm{out}} =& \boldsymbol{H}(\boldsymbol{N}_{\mathrm{H}} + \boldsymbol{N}_4)\boldsymbol{H}^{\mathrm{T}} + \boldsymbol{M}_4(\boldsymbol{N}_{\mathrm{J}} + \boldsymbol{N}_3)\boldsymbol{M}_4^{\mathrm{T}} + \boldsymbol{M}_3\boldsymbol{N}_2\boldsymbol{M}_3^{\mathrm{T}} + \boldsymbol{M}_2\boldsymbol{N}_1\boldsymbol{M}_2^{\mathrm{T}},\\ \boldsymbol{M}_2 =& \boldsymbol{H}\boldsymbol{L}_4\boldsymbol{J}_{\mathrm{B}}\boldsymbol{L}_3\boldsymbol{C}_{\mathrm{E}}\boldsymbol{L}_2\boldsymbol{C}_{\mathrm{A}},\\ \boldsymbol{M}_3 =& \boldsymbol{H}\boldsymbol{L}_4\boldsymbol{J}_{\mathrm{B}}\boldsymbol{L}_3\boldsymbol{C}_{\mathrm{E}},\\ \boldsymbol{M}_4 =& \boldsymbol{H}\boldsymbol{L}_4\boldsymbol{J}_{\mathrm{B}}.\end{aligned} \tag{S27}$$

Based on our model in Eq. S26, we can describe the result of individual SQMs performed by Bob by computing the mean value and variance of the quadrature amplified by phase-sensitive amplification. This quadrature can be readily extracted from the first two diagonal elements of $\boldsymbol{V}_{\mathrm{out}}$. For a symbol $\alpha_i$ of Alice, we obtain from our model that Bob's individual SQM, resulting in a measured symbol $\beta_i$, can be described by a Gaussian random variable with mean $\mu_{\mathrm{B|A}}$ and variance $\sigma^2_{\mathrm{B|A}}$. In order to write their expression in a compact analytical form, we introduce the notation

$$\tau_i = 1 - \varepsilon_i, \quad i \in \{1, 2, 3, 4\}. \tag{S28}$$

Using Eqs. S26 and S28, we obtain

$$\begin{aligned}\mu_{\mathrm{B|A}} &= \sqrt{G_{\mathrm{H}}}\sqrt{G_{\mathrm{J}}}\sqrt{\tau_{\mathrm{tot}}}\alpha_i = \sqrt{G_{\mathrm{H}}}\sqrt{G_{\mathrm{J}}}\,\beta_i,\\ \sigma^2_{\mathrm{B|A}} &= G_{\mathrm{H}}\left[G_{\mathrm{J}}\left(\sigma_{\mathrm{n}}^2 + N_{\mathrm{X}}\right)\right],\end{aligned} \tag{S29}$$

where we have defined

$$\begin{aligned}
\sigma_{\mathrm{n}}^{2} &= \tau_{\mathrm{tot}}\sigma_{\mathrm{s}}^{2} + \frac{1}{4}\tau_{\mathrm{th}}\left(1+2\bar{n}_{\mathrm{th}}\right) + \tau_{4}\tau_{3}\left(\frac{1}{4}\varepsilon_{\mathrm{E}} + \bar{n}\right), \\
N_{\mathrm{X}} &= \tau_{4}\frac{\bar{n}_{\mathrm{J}}}{2} + \frac{\bar{n}_{\mathrm{H}}}{2G_{\mathrm{J}}}, \\
\tau_{\mathrm{tot}} &= \tau_{1}\tau_{2}\tau_{\mathrm{A}}\tau_{3}\tau_{\mathrm{E}}\tau_{4}, \\
\tau_{\mathrm{th}} &= \tau_{4}\tau_{3}\tau_{\mathrm{E}}\left(1-\tau_{2}\tau_{\mathrm{A}}\tau_{1}\right) + \tau_{4}\varepsilon_{3}, \\
\bar{n} &= \frac{\varepsilon_{\mathrm{E}}\bar{n}_{\mathrm{E}}}{2}.
\end{aligned} \tag{S30}$$

We note that during measurements, the value of $\beta_i = \sqrt{\tau_{\mathrm{tot}}}\,\alpha_i$ can be computed by rescaling the measured symbols by $\sqrt{G_{\mathrm{H}}}\sqrt{G_{\mathrm{J}}}$. The individual values of $G_{\mathrm{H}}$ and $G_{\mathrm{J}}$ are obtained from calibration measurements (see Sec. VI A and Sec. VI D). To compute the overall statistics of Bob's key, we recall that the indistinguishability between the two quadratures imposes the condition

$$\sigma_{\mathrm{s}}^{2} + \sigma_{\mathrm{A}}^{2} = \sigma_{\mathrm{as}}^{2}. \tag{S31}$$

The mean and variance of the distribution of Bob's key can be viewed as a convolution between the Gaussian modulation of Alice's symbols and the Gaussian quadrature distribution of Bob's individual states. As such, we compute Bob's key probability density function $f_{\mathrm{B}}$ as

$$f_{\mathrm{B}}\left(y\right) = \int_{-\infty}^{\infty} f_{\mathrm{B|A}}\left(x\right) f_{\mathrm{A}}\left(x\right) dx, \tag{S32}$$

where $f_{\mathrm{B|A}}$ is the the probability density function of Bob's individual SQMs and $f_{\mathrm{A}}$ is the probability density function of Alice's Gaussian distribution. As a result, Bob's measured key has also a Gaussian distribution with a mean $\mu_{\mathrm{B}}$ and a variance $\sigma_{\mathrm{B}}^{2}$ given by

$$\begin{aligned}
\mu_{\mathrm{B}} &= 0, \\
\sigma_{\mathrm{B}}^{2} &= G_{\mathrm{H}}\left[G_{\mathrm{J}}\left(\tau_{\mathrm{tot}}\sigma_{\mathrm{as}}^{2} + \frac{1}{4}\tau_{\mathrm{th}}\left(1+2\bar{n}_{\mathrm{th}}\right) + \tau_{3}\tau_{4}\left(\frac{1}{4}\tau_{\mathrm{E}} + \bar{n}\right) + \tau_{4}\frac{\bar{n}_{\mathrm{J}}}{2}\right) + \frac{\bar{n}_{\mathrm{H}}}{2}\right].
\end{aligned} \tag{S33}$$

We emphasize that the experimentally measured values are rescaled by the gains values $G_{\mathrm{H}}$ and $G_{\mathrm{J}}$ during data analysis of Bob's keys.

## III. TEST OF NORMALITY

To verify the Gaussianity of the measured keys, we rely on a well-known normality test, namely the Shapiro–Wilk (SW) test. We additionally use two other common tests, the Anderson–Darling (AD) test and the Jarque–Bera (JB) test, to confirm the validity of the first test. Each test presents some robustness compared to the others. They are designed to test the validity of a null hypothesis as compared to an alternative hypothesis (the negation of the null hypothesis most often). For these tests, the null hypothesis consists of stating that the observed data is normally distributed. For a given test, a so-called *p-value* is computed which indicates the likelihood of the observed data to have occurred under the null hypothesis. One defines a confidence threshold $\alpha_{\mathrm{thres}}$ and the null hypothesis can be rejected in the case of $p$-value $< \alpha_{\mathrm{thres}}$. To reject the null

hypothesis, we note that a small p-value has to be obtained, where one would have to compute typically a $p$-value $\leq 0.05$. One commonly considers that a $p$-value $\geq 0.1$ does not provide evidence against the null hypothesis.

The SW test typically presents a high probability of rejecting the null hypothesis given that the alternative hypothesis is true [S4]. The AD test is a commonly used test to evaluate observed data for any given probability distributions, not necessarily restricted to normal distributions [S4]. Lastly, the JB test can be used to test for normality of observed data by verifying whether or not the data skewness and kurtosis match a normal distribution [S4]. Similarly to the SW test, the JB test presents a high probability of rejecting the null hypothesis under the assumption that the alternative hypothesis is true. The JB test is more suited than the SW test for a large data set of samples. More precisely, the SW test is recommended for a data set of less than 5000 samples. Since our sample size does not differ greatly from this threshold, we decide to include both the SW and JB test.

All tests are performed using the Statistics Toolbox of the programming language MATLAB®. For all three tests and for all keys, we obtain a $p$-value of at least $0.1$. Thus, we conclude that there is no statistical evidence to reject the null hypothesis and, as a result, we can consider that our measured keys are distributed according to Gaussian distributions. This result is in agreement with the assumption that all contributions of the variance of Bob presented in Eq. S33 have a Gaussian distribution. In particular, this result is in agreement with the fact that our measurement JPA, which we assume to perform a phase-sensitive amplification, behaves as a linear amplifier throughout the measurements.

## IV. COMPARISON MODEL AND MEASUREMENT

We use the Bhattacharyya coefficient $\mathcal{B}$ between measured quadrature distribution and our corresponding model prediction introduced in Eq. S33. For continuous variables, the coefficient $\mathcal{B}$ is defined as

$$\mathcal{B}\left(P_1, P_2\right) = \int_{\mathcal{D}} \sqrt{P_1\left(x\right) P_2\left(x\right)}\, dx, \tag{S34}$$

where $P_1$ and $P_2$ are two probability density functions and $\mathcal{D}$ is a common domain of definition. For Gaussian random variables where the domain of definition is the entire real axis, the coefficient results in the simple form

$$\mathcal{B}\left(P_1, P_2\right) = \sqrt{\frac{2\sigma_1\sigma_2}{\sigma_1^2 + \sigma_2^2}} \exp\left(-\frac{1}{4}\frac{\left(\mu_1 - \mu_2\right)^2}{\sigma_1^2 + \sigma_2^2}\right), \tag{S35}$$

where $\mu_1$ and $\mu_2$ are the mean values of the Gaussian distributions $P_1$ and $P_2$, respectively. Similarly, $\sigma_1$ and $\sigma_2$ are the standard deviations of the Gaussian distributions. By definition, we have $0 \leq \mathcal{B} \leq 1$. Thus, the coefficient $\mathcal{B}$ quantifies an overlap between the distributions $P_1$ and $P_2$. The Bhattacharyya coefficient can be used to define a proper metric for probability density functions, called the Hellinger distance

$$H\left(P_1, P_2\right) = \sqrt{1 - \mathcal{B}\left(P_1, P_2\right)}, \qquad 0 \leq H \leq 1. \tag{S36}$$

Since $H$ is a distance, it fulfils the triangular inequality and, in particular, we have the property $H\left(P_1, P_2\right) = 0 \Leftrightarrow P_1 = P_2$. It follows that the closer the Hellinger distance is to zero, the

closer the probability density functions $P_1$ and $P_2$ are to each other. Equivalently, the closer the Bhattacharyya coefficient is to unity, the closer the probability density functions $P_1$ and $P_2$ are to each other. According to Sec. III, we can consider that our measured keys are distributed according to Gaussian distributions, and we evaluate the relevant Bhattacharyya coefficients with associated Hellinger distances using Eqs. S35 and S36.

## V. MUTUAL INFORMATION

The mutual information between Alice's and Bob's keys can be written using the differential entropy as

$$I\left(\mathcal{K}_{\mathrm{A}} \colon \mathcal{K}_{\mathrm{B}}\right) = h\left(\mathcal{K}_{\mathrm{B}}\right) - h\left(\mathcal{K}_{\mathrm{B}}|\mathcal{K}_{\mathrm{A}}\right), \tag{S37}$$

where $h$ is the differential entropy. For a Gaussian variable $X$, the differential entropy, expressed in bits, simplifies to

$$h\left(X\right) = \frac{1}{2}\log_2\left(2\pi e\,\sigma_{\mathrm{X}}^2\right), \tag{S38}$$

where $\sigma_{\mathrm{X}}^2$ is the variance of the random variable $X$. One can show that

$$\sigma_{\mathrm{B|A}}^2 = \sigma_{\mathrm{B}}^2 - \frac{\mathrm{Cov}(\mathcal{K}_{\mathrm{A}}, \mathcal{K}_{\mathrm{B}})^2}{\sigma_{\mathrm{A}}^2}, \tag{S39}$$

where $\mathrm{Cov}(\mathcal{K}_{\mathrm{A}}, \mathcal{K}_{\mathrm{B}})$ is the classical covariance between Alice's key $\mathcal{K}_{\mathrm{A}}$ and Bob's key $\mathcal{K}_{\mathrm{B}}$. This results in the expression for the mutual information

$$I\left(\mathcal{K}_{\mathrm{A}} \colon \mathcal{K}_{\mathrm{B}}\right) = \frac{1}{2}\log_2\left(\frac{\sigma_{\mathrm{A}}^2\,\sigma_{\mathrm{B}}^2}{\sigma_{\mathrm{A}}^2\,\sigma_{\mathrm{B}}^2 - \mathrm{Cov}(\mathcal{K}_{\mathrm{A}}, \mathcal{K}_{\mathrm{B}})^2}\right) = \frac{1}{2}\log_2\left(1 + \frac{\mathrm{Cov}(\mathcal{K}_{\mathrm{A}}, \mathcal{K}_{\mathrm{B}})^2}{\sigma_{\mathrm{A}}^2\,\sigma_{\mathrm{B}}^2 - \mathrm{Cov}(\mathcal{K}_{\mathrm{A}}, \mathcal{K}_{\mathrm{B}})^2}\right). \tag{S40}$$

Here, we define the signal-to-noise ratio as $\mathrm{SNR} = \mathrm{Cov}(\mathcal{K}_{\mathrm{A}}, \mathcal{K}_{\mathrm{B}})^2/(\sigma_{\mathrm{A}}^2\,\sigma_{\mathrm{B}}^2 - \mathrm{Cov}(\mathcal{K}_{\mathrm{A}}, \mathcal{K}_{\mathrm{B}})^2)$. The last result in Eq. S40 offers a direct practical implementation as it provides a direct computation of the mutual information from our measured keys. Using Eqs. S29 and S33, we can calculate the corresponding mutual information from our quadrature distribution model, resulting in

$$\begin{aligned} I\left(\mathcal{K}_{\mathrm{A}} \colon \mathcal{K}_{\mathrm{B}}\right) &= \frac{1}{2}\log_2\left(\frac{\sigma_{\mathrm{B}}^2}{\sigma_{\mathrm{B|A}}^2}\right) \\ &= \frac{1}{2}\log_2\left(1 + \frac{\tau_{\mathrm{tot}}\sigma_{\mathrm{A}}^2}{\tau_{\mathrm{tot}}\sigma_{\mathrm{s}}^2 + \tau_{\mathrm{th}}\left(1 + 2\bar{n}_{\mathrm{th}}\right)/4 + \tau_3\tau_4\left(\varepsilon_{\mathrm{E}}/4 + \bar{n}\right) + \tau_4\bar{n}_{\mathrm{J}}/2 + \bar{n}_{\mathrm{H}}/(2G_{\mathrm{J}})}\right). \end{aligned} \tag{S41}$$

Each term in Eq. S41 can be obtained from independent calibration measurements, which we detail in the following sections. Using these calibration measurements, we can compare the value of the mutual information predicted by our model in Eq. S41 and the mutual information calculated from measured keys using Eq. S40.

## VI. CALIBRATION MEASUREMENTS

### A. Photon number calibration

In our measurements, we perform a photon number calibration of our detection chain using a two-dimensional Planck spectroscopy [S5]. During this measurement, both JPAs are far detuned from resonance. To implement the Planck spectroscopy, we use a heatable $30\,\mathrm{dB}$ attenuator at the input of our cryogenic setup, serving as a self-calibrated reference thermal photon source, which we can controllably heat up to a desired setpoint temperature $T_{\mathrm{att}}$. This attenuator is weakly thermally anchored to the mixing chamber stage of our dilution refrigerator. We controllably vary the temperature of the mixing chamber to the setpoint temperature $T_{\mathrm{mc}}$. For each chosen temperature of the mixing chamber stage $T_{\mathrm{mc}}$, we sweep the temperature of our heatable attenuator in a temperature range varying from a base temperature slightly above $T_{\mathrm{mc}}$ to a final temperature $T_{\mathrm{att}} = 440\,\mathrm{mK}$. This procedure allows for a precise extraction of the losses, $\tau_{2\mathrm{D}}$, between the heatable attenuator and the input of the HEMT. According to ref. S5, the measured power $P$ at the end of our detection chain reads

$$P = \frac{\kappa}{Z_0}\left[\frac{\tau_{2\mathrm{D}}}{2}\coth\left(\frac{\hbar\omega}{2k_{\mathrm{B}}T_{\mathrm{att}}}\right) + \frac{1-\tau_{2\mathrm{D}}}{2}\coth\left(\frac{\hbar\omega}{2k_{\mathrm{B}}T_{\mathrm{mc}}}\right) + \bar{n}_{\mathrm{amp}}\right], \tag{S42}$$

where $\kappa$ is the photon number conversion factor (PNCF) relating the measured power to the photon number at the input of the HEMT. Furthermore, the photon number $\bar{n}_{\mathrm{amp}}$ is the number of noise photons added by our amplification chain, with the main noise contribution coming from the cryogenic HEMT. Since the HEMT is operated with a gain $G_{\mathrm{H}} = 43\,\mathrm{dB}$, we neglect the subsequent noise contributions from additional room temperature amplifiers. Therefore, without loss of information, in our analysis we use $\bar{n}_{\mathrm{H}} = \bar{n}_{\mathrm{amp}}$. Lastly, $Z_0$ corresponds to the characteristic $50\,\Omega$ impedance of our microwave circuits. As shown in Fig. S3, we fit all the results of Planck spectroscopy at once according to Eq. S42 to determine $\tau_{2\mathrm{D}}$, $\kappa$, and $\bar{n}_{\mathrm{amp}}$. In our quadrature distribution model, we need to consider losses in our setup from the first JPA to the input of the HEMT, $\tau_{\mathrm{tot}}$. To this end, we carefully estimate the losses between the heatable attenuator and the first JPA, $\tau_0$, and compute $\tau_{\mathrm{tot}} = \tau_{2\mathrm{D}}/\tau_0 = 0.5785$.

### B. Squeezing and displacement calibration

We reconstruct squeezed states generated by the first JPA when pumped at twice their resonance frequency using the reference-state reconstruction method. In particular, we calculate squeezing and anti-squeezing variances based on reconstructed signal moments $\langle (a^\dagger)^n a^m \rangle$. During this measurement, the measurement JPA is detuned from resonance and other devices except for the JPA pump are not active. For a given pump power, we extract the variance of the *q* and *p* quadratures from the reconstructed signal moments using

$$\begin{aligned}
\sigma_q^2 &= \frac{\langle \hat{a}^2\rangle + \langle(\hat{a}^\dagger)^2\rangle + 2\langle \hat{a}^\dagger\hat{a}\rangle + 1}{4} - \frac{\langle \hat{a}\rangle^2 + \langle(\hat{a}^\dagger)\rangle^2 + 2\langle \hat{a}^\dagger\rangle\langle \hat{a}\rangle}{4}, \\
\sigma_p^2 &= \frac{\langle \hat{a}^2\rangle + \langle(\hat{a}^\dagger)^2\rangle - 2\langle \hat{a}^\dagger\hat{a}\rangle + 1}{4} - \frac{\langle \hat{a}\rangle^2 + \langle(\hat{a}^\dagger)\rangle^2 - 2\langle \hat{a}^\dagger\rangle\langle \hat{a}\rangle}{4}.
\end{aligned} \tag{S43}$$

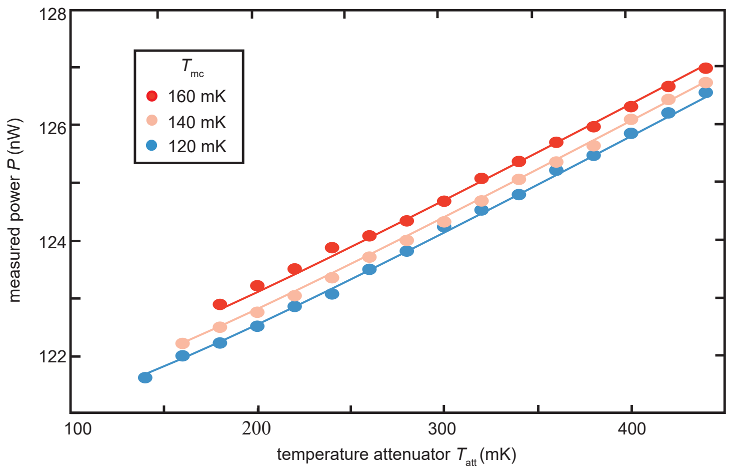


Figure S3. Experimental two-dimensional Planck spectroscopy of our microwave setup. Symbols depict experimental data and solid lines are corresponding fits according to Eq. S42. The losses extracted from the measurement are $\tau_{\mathrm{2D}} = 0.4941$, corresponding to losses $L_{\mathrm{2D}} = -10\log(\tau_{\mathrm{2D}}) = 3.07\,\mathrm{dB}$.

Considering that we are restricted to $q$ or $p$ squeezed state, the squeezed quadrature variance is obtained as $\sigma_{\mathrm{s}}^2 = \min(\sigma_q^2, \sigma_p^2)$. The anti-squeezed quadrature variance is similarly computed as $\sigma_{\mathrm{as}}^2 = \max(\sigma_q^2, \sigma_p^2)$. In our work, we keep a constant squeezing level $S = 3.6\,\mathrm{dB}$ corresponding to $\sigma_{\mathrm{s}}^2 = 0.11$. Simultaneously, the modulation variance is extracted according to $\sigma_{\mathrm{s}}^2 + \sigma_{\mathrm{A}}^2 = \sigma_{\mathrm{as}}^2$. For the 1st run, we obtain $\sigma_{\mathrm{A}}^2 = \sigma_{\mathrm{as}}^2 - \sigma_{\mathrm{s}}^2 = 1.17$ and, for the 2nd run, $\sigma_{\mathrm{A}}^2 = 1.33$.

Following a similar procedure, we calibrate the displacement induced from coupling a strong coherent tone to incoming signals through the first directional coupler. To this end, we vary the power of the coherent tone $P_{\mathrm{coh}}$ and reconstruct a displacement photon number $\bar{n}_{\mathrm{disp}} = \langle \hat{a}^\dagger \hat{a} \rangle$ at the output of the first directional coupler using the reference-state reconstruction method. The measured values can be linearly fitted as $\bar{n}_{\mathrm{disp}} = m\,P_{\mathrm{coh}} + p$, where $m$ and $p$ are two fit parameters. From this fit, we can reliably convert any symbol $\alpha_i$ of Alice's key into a corresponding power $P_i$ to set for the coherent tone according to

$$P_i = \frac{|\alpha_i|^2 - p}{m}. \tag{S44}$$

### C. Coupled noise calibration

The coupled noise photon number $\bar{n}$ is extracted from a measurement with only the noise source being active. During this measurement, the JPAs are detuned far from resonance by several dozens of megahertz. We relate the reconstructed photon number $\bar{n}_{\mathrm{n}} = \left\langle \hat{a}^\dagger \hat{a} \right\rangle$ at the input of the HEMT to the noise photon number $\bar{n}_{\mathrm{E}}$ at the input of the coupling port of the second directional coupler. Considering that the final measured state corresponds to a thermal state, we derive the relation

$$(\tau_4\tau_3\tau_{\mathrm{E}} + 1 - \tau_3\tau_4)\,(1 + 2\bar{n}_{\mathrm{th}}) + \tau_3\tau_4\varepsilon_{\mathrm{E}}\,(1 + 2\bar{n}_{\mathrm{E}}) = (1 + 2\bar{n}_{\mathrm{n}})\,. \tag{S45}$$

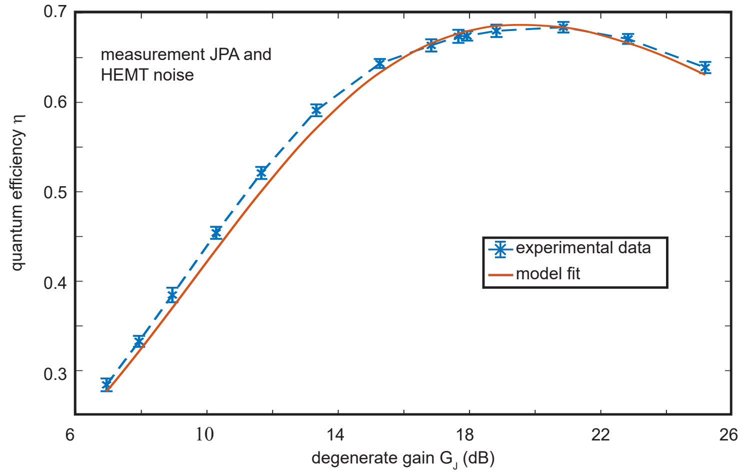


Figure S4. Experimental quantum efficiency accounting for the noise of the second flux-driven JPA and for the HEMT noise. The quantum efficiency is plotted as a function of the degenerate amplification gain $G_{\rm J}$ of the measurement JPA. The measurement is performed for displaced squeezed states as input states to the measurement JPA. The blue symbols correspond to measured data with the blue dashed line serving as a guide to the eye. The orange solid line is obtained from a model fit according to Eqs. S8 and S50.

This equation can be reformulated to separate the losses and the noise contribution as

$$\frac{(\tau_4\tau_3\tau_{\rm E}+1-\tau_3\tau_4)\,(1+2\bar{n}_{\rm th})+\tau_3\tau_4\varepsilon_{\rm E}}{4}+\tau_3\tau_4\bar{n}=\frac{(1+2\bar{n}_{\rm n})}{4}, \tag{S46}$$

where we have defined the coupled noise photon number

$$\bar{n}=\frac{\varepsilon_{\rm E}\bar{n}_{\rm E}}{2}. \tag{S47}$$

As a result, we can extract a coupled noise photon number from the measurement given by

$$\bar{n}=\frac{\bar{n}_{\rm n}-(\tau_4\tau_3\tau_{\rm E}+1-\tau_4\tau_3)\,\bar{n}_{\rm th}}{2\tau_4\tau_3}. \tag{S48}$$

To determine $\bar{n}$, we experimentally vary the total reconstructed photon number $\bar{n}_{\rm n}$ by sweeping the power of the noise source $P_{\rm n}$. The measured values can be linearly fitted according to $\bar{n}_{\rm n} = m'\,P_{\rm n}+p'$, where $m'$ and $p'$ are two fit parameters, similarly to the displacement photon number calibration. From Eq. S48, we can reliably convert a given photon number $\bar{n}$ into a corresponding power $P_{\rm n}$.

### D. Quantum efficiency calibration

In Fig. S4, we plot the measured quantum efficiency $\eta$ as a function of the measurement JPA degenerate amplification gain $G_{\rm J}$. We extract the quantum efficiency from a measurement with all devices being active (except for the noise source) and with the JPAs tuned into resonance. This implies that we generate displaced squeezed states which we subsequently phase-sensitively amplify. We choose to amplify along the $q$ or $p$ quadrature and record the power, $P_{\rm amp}$, for the amplified

quadrature from first order signal moment, i.e., $P_{\mathrm{amp}} = (\kappa/Z_0)\langle\hat{q}\rangle^2$ or $P_{\mathrm{amp}} = (\kappa/Z_0)\langle\hat{p}\rangle^2$. Here, $\kappa$ is the PNCF. As a power reference, we use the measured power $P_{\mathrm{ref}}$, detected by performing the exact same measurement but without pumping the measurement JPA. This provides an *in situ* degenerate-gain measurement $G_{\mathrm{J}} = P_{\mathrm{amp}}/P_{\mathrm{ref}}$. Additionally, we extract from this measurement a value for the added noise photon number $\bar{n}_{\mathrm{H}}/2$ to the quadrature. This photon number is measured during a measurement window where no devices are active (required for our reference-state reconstruction method). We extract the noise variance $N_{\mathrm{X}}$ added to the amplified quadrature as

$$N_{\mathrm{X}} = \frac{\sigma^2_{\mathrm{tot}}}{G_{\mathrm{H}}\,G_{\mathrm{J}}} - \sigma^2_{\mathrm{n}}. \tag{S49}$$

Here, $\sigma^2_{\mathrm{tot}} = \sigma^2_{\mathrm{B|A}}\left(\bar{n} = \varepsilon_{\mathrm{E}}\bar{n}_{\mathrm{th}}/2\right)$ is the reconstructed variance of the amplified quadrature with all components active (except for the noise source), where we are also accounting for the HEMT noise contribution. We simultaneously extract the variance $\sigma^2_{\mathrm{n}}$ by reconstructing the variance of the to-be-amplified quadrature, while the pump of the measurement JPA is switched off. The quantum efficiency is defined as

$$\eta = \frac{1}{1 + 2[N_{\mathrm{X}} - 1/(4\,G_{\mathrm{J}})]} = \frac{1}{1 + 2\bar{n}_{\mathrm{X}}}. \tag{S50}$$

We fit the measured quantum efficiency according to Eqs. S8 and S50 and display the resulting fit in Fig. S4. The fit is performed by minimizing the difference between the measured quantum efficiencies and their corresponding model prediction using a nonlinear solver under constraints of the Optimization Toolbox of MATLAB®. The resulting fit values are $\Xi_1 = 0.048$ and $\Xi_2 = 0.42$.

### Parameter estimation and finite-size terms

Alice and Bob estimate the losses and coupled noise photon number of the quantum channel by building statistical unbiased estimators from a publicly disclosed fraction of length $m = N - n_{\mathrm{ec}}$ of their exchanged key. Using the disclosed data, a square root transmissivity unbiased estimator can be constructed as [S6]

$$\hat{T}_{\mathrm{tot}} = \frac{\sum_{i=1}^{m}\left(\alpha_i - \bar{A}\right)\left(\beta_i - \bar{B}\right)}{\sum_{i=1}^{m}\left(\alpha_i - \bar{A}\right)^2}, \tag{S51}$$

where we denote $\bar{A}$ as the average value of Alice's key $\mathcal{K}_{\mathrm{A}} = \{\alpha_i\}_{i\in\{1,\cdots,N\}}$ while $\bar{B}$ denotes the average value of Bob's key $\mathcal{K}_{\mathrm{B}} = \{\beta_i\}_{i\in\{1,\cdots,N\}}$. From this estimator, we define the new estimator $\hat{\tau}_{\mathrm{tot}} = \hat{T}^2_{\mathrm{tot}}$. This estimator is unbiased since $\langle\hat{\tau}_{\mathrm{tot}}\rangle = \tau_{\mathrm{tot}}$. According to Eq. S30, we obtain an unbiased estimator of $\varepsilon_{\mathrm{E}}$ as $\hat{\varepsilon}_{\mathrm{E}} = 1 - \hat{\tau}_{\mathrm{E}} = 1 - \hat{\tau}_{\mathrm{tot}}/(\tau_1\tau_2\tau_{\mathrm{A}}\tau_3\tau_4)$. From the previous result, we can construct an unbiased estimator for the total noise photon number [S6]

$$\hat{\bar{n}}_{\mathrm{tot}} = \frac{1}{m}\sum_{i=1}^{m}\left(\beta_i - \hat{T}_{\mathrm{tot}}\,\alpha_i\right)^2. \tag{S52}$$

This estimator converges to the total noise photon number, which we relate to the coupled noise photon number using $\langle\hat{\bar{n}}_{\mathrm{tot}}\rangle = \bar{n}_{\mathrm{tot}} = \tau_{\mathrm{tot}}\sigma^2_{\mathrm{s}} + \tau_{\mathrm{th}}\left(1 + 2\bar{n}_{\mathrm{th}}\right)/4 + \tau_4\tau_3\left(\varepsilon_{\mathrm{E}}/4 + \bar{n}\right) + N_{\mathrm{X}}$. We compute a worst-case scenario unbiased estimator of the losses considering a confidence parameter

$w$ such that

$$\varepsilon_{\mathrm{E}}^{\star} = \hat{\varepsilon}_{\mathrm{E}} - w\,\sigma_{\hat{\varepsilon}_{\mathrm{E}}} \simeq \hat{\varepsilon}_{\mathrm{E}} - 2w\sqrt{\left(\frac{\bar{n}_{\mathrm{tot}}}{\sigma_{\mathrm{A}}^{2}} + 2\tau_{\mathrm{tot}}\right)\frac{\tau_{\mathrm{E}}}{m}}. \tag{S53}$$

For Gaussian random variables, the confidence parameter $w$ reduces to the simple form

$$w = \sqrt{2}\,\mathrm{erf}^{-1}\left(1 - 2\varepsilon_{\mathrm{ec}}\right), \tag{S54}$$

with $\varepsilon_{\mathrm{ec}}$ defined as an error probability, typically set in the range of $10^{-10}$ for CV-QKD protocols [S6]. This gives the common value of $w \simeq 6.34$. We can further extend this analysis to obtain a worst-case scenario unbiased estimator of the coupled noise photon number. First, we define an unbiased coupled noise photon number estimator

$$\hat{\bar{n}} = \hat{\bar{n}}_{\mathrm{tot}} - \hat{\tau}_{\mathrm{tot}}\,\sigma_{\mathrm{s}}^{2} - \tau_{\mathrm{th}}\left(1 + 2\bar{n}_{\mathrm{th}}\right)/4 - \tau_{3}\tau_{4}\frac{\varepsilon_{\mathrm{E}}^{\star}}{4} - N_{\mathrm{X}}. \tag{S55}$$

This results in the worst-case scenario unbiased estimator for the coupled noise photon number

$$\bar{n}^{\star} = \hat{\bar{n}} + w\,\sigma_{\hat{\bar{n}}} \simeq \hat{\bar{n}} + w\sqrt{\frac{\bar{n}_{\mathrm{tot}}^{2}}{8\,m}}. \tag{S56}$$

Since a part of the secret key must be used for parameter estimation, Alice and Bob only preserve a key of finite size $n_{\mathrm{ec}} = N - m$ at the end of the error reconciliation step. In this work, we vary the fraction $m$ to optimize the precision of our worst-case scenario estimators. The finite-size terms appearing in the finite-size secret key bound are calculated as [S6]

$$\begin{aligned} \Delta\left(n_{\mathrm{exp}}\right) &= \frac{\Delta_{\mathrm{fs}}}{\sqrt{n_{\mathrm{ec}}}} - \frac{\Theta}{n_{\mathrm{ec}}}, \\ \Delta_{\mathrm{fs}} &= 4\log_{2}\left(\sqrt{d} + 2\right)\sqrt{\log_{2}\left(\frac{18}{p_{\mathrm{ec}}^{2}\varepsilon_{\mathrm{s}}^{4}}\right)}, \\ \Theta &= \log_{2}\left[p_{\mathrm{ec}}\left(1 - \frac{\varepsilon_{\mathrm{s}^2}}{3}\right)\right] + 2\log_{2}\left(\sqrt{2}\,\varepsilon_{\mathrm{h}}\right). \end{aligned} \tag{S57}$$

Here, the parameter $d$ represents the dimension of Alice's and Bob's effective codebook after a discretization step during error reconciliation. This discretization is required to transform their data from a continuous set into a discrete set over which existing classical optimized error correction algorithm can be run. We consider a typical value for CV-QKD protocols of $d = 2^{5}$ for a 5-bit discretization. The overall success of the protocol is limited by the tolerance error for the security of the protocol, reflected in a smoothing parameter $\varepsilon_{\mathrm{s}}$ and a hashing parameter $\varepsilon_{\mathrm{h}}$. These parameters determine the total error of the privacy amplification step, which follows the error correction step. The goal of privacy amplification is to remove remaining information of Eve about Alice's and Bob's error corrected key. In this work, we choose an illustrative value of $\varepsilon_{\mathrm{s}} = \varepsilon_{\mathrm{h}} = 10^{-3}$, although we note that conservative values of $\varepsilon_{\mathrm{s}} = \varepsilon_{\mathrm{h}} = 10^{-10}$ are typically chosen for CV-QKD protocol [S6]. We emphasize that this point does not change our conclusion from the main text regarding the finite-size terms. In particular, the conclusion regarding the increase of the sample size to $N \geq 10^{6}$ remains valid for $\varepsilon_{\mathrm{s}} = \varepsilon_{\mathrm{h}} = 10^{-10}$. Lastly, one can consider realistic values of

0.95 for both the efficiency of the error correction $\beta$ with associated success probability $p_{\mathrm{ec}}$.

---


[S1] K. G. Fedorov, S. Pogorzalek, U. Las Heras, M. Sanz, P. Yard, P. Eder, M. Fischer, J. Goetz, E. Xie, K. Inomata, Y. Nakamura, R. Di Candia, E. Solano, A. Marx, F. Deppe, and R. Gross, Finite-time quantum entanglement in propagating squeezed microwaves, Sci. Rep. **8**, 6416 (2018).

[S2] S. Pogorzalek, K. G. Fedorov, M. Xu, A. Parra-Rodriguez, M. Sanz, M. Fischer, E. Xie, K. Inomata, Y. Nakamura, E. Solano, *et al.*, Secure quantum remote state preparation of squeezed microwave states, Nat. Commun. **10**, 2604 (2019).

[S3] C. Eichler, D. Bozyigit, C. Lang, M. Baur, L. Steffen, J. M. Fink, S. Filipp, and A. Wallraff, Observation of two-mode squeezing in the microwave frequency domain, Phys. Rev. Lett. **107**, 113601 (2011).

[S4] M. Lovric, *International Encyclopedia of Statistical Science* (Springer, Berlin, 2011).

[S5] S. Gandorfer, M. Renger, W. K. Yam, F. Fesquet, A. Marx, R. Gross, and K. G. Fedorov, Two-dimensional planck spectroscopy, Preprint at `https://arxiv.org/abs/2308.02389` (2023).

[S6] S. Pirandola, Composable security for continuous variable quantum key distribution: Trust levels and practical key rates in wired and wireless networks, Phys. Rev. Res. **3**, 043014 (2021).
